# Supplementary material for: LocalTweets to LocalHealth: A Mental Health Surveillance Framework Based on Twitter Data
Source: arXiv:2402.13452 source file (2024-03-26)
Supplement: Supplementary file 1 [file table_appendix_northeast.tex]

% table_appendix_northeast.tex

\begin{table}[h]

\centering
\begin{tabularx}{\linewidth}{Xccc}
\toprule
\textbf{Input information} & \textbf{F1-score} & \textbf{Acc. (\%)} \\
\midrule

\multicolumn{3}{p{7cm}}{\textbf{Text-based (LocalHealth) with ADI}} \\ % & & & & \\
MH-only & 0.7514 & 75.67 \\
FI only & 0.7503 & 75.52 \\
MH and FI & 0.7560 & 76.02 \\
General only & 0.7450 & 75.09 \\

\bottomrule
\end{tabularx}

\caption{\textbf{Effect of Under Representation of Northeast Region.} 
}
\label{table:appendix_northeast}

\end{table}
